# Supplementary material for: Reachability and Matching in Single Crossing Minor Free Graphs
Source: arXiv:2103.13940 source file (2021-09-04)
Supplement: Supplementary file 1 [file isoAppendix.tex]

\section{The details from Section~\ref{sec:iso}}\label{subsec:isoApp}
We use the same general strategy as in \cite{DKMTVZ20} and divide the edges into
\emph{real} and \emph{fictitious} where the former represent the newly inserted
edges and the latter original undeleted edges\footnote{We use the terms
old $\leftrightarrow$ fictitious and new $\leftrightarrow$ real interchangeably
in this section.}.

Let $\calC$ be a set of cycles containing both real and fictitious edges that 
occur in any PM. %Let $\calC$ be the corresponding set
%system where all fictitious edges have been deleted. 
Let $w$ be a  weight 
function on the edges that gives non-zero weight only to the real edges.
Define $c_w(\calC)$ to be the set of all circulations in the cycles of 
$\calC$. Here the circulation is the absolute value of the alternating sum
of weights $c_w(C) = |w(f_1) - w(f_2) + w(f_3) - \ldots|$ where 
$C = f_1,f_2,f_3,\ldots$ is the sequence of edges in the cycle. 

We say that a weight function,
that gives non-zero weights to the real edges, \emph{real isolates} $\mathcal{M}$ 
for a set system $\mathcal{M}$ if the minimum weight set in $\mathcal{M}$ is unique. In our context $\mathcal{M}$ will refer to the set of perfect/maximum
 matchings.

Next we follow the proof idea of \cite{FGT} but focus on assigning weights
to real edges which are, say, $N$ in number.
 We do this in $\log{N}$ stages starting with a graph $G_0 = G$
and ending with the acyclic graph $G_\ell$ where $\ell = \log{N}$. The inductive
assumption is that:
\begin{invariant}\label{inv:analogFGT}
 For $i \geq 1$, $G_i$ contains no cycles with at most $2^{i+1}$ real edges. 
\end{invariant}

Notice that induction starts at $i > 0$.
%Initially, this is trivially true for $G_0$.

We first show how to construct $G_{i+1}$ from $G_i$ such that if $G_i$ satisfies
the inductive invariant~\ref{inv:analogFGT} then so does $G_{i+1}$.
Let $i > 1$, then in the $i$-th stage, let $\calC_{i+1}$ be the set of cycles that contain 
%(at least $2^i$) and 
at most $2^{i+2}$ real edges. For each such cycle 
$C = f_0,f_1,\ldots$ containing $k \leq 2^{i+2}$ real edges (with $f_0$ being the
least numbered real edge in the cycle) edge-partition it into $4$ consecutive 
paths $P_j(C)$ for $j \in \{0,1,2,3\}$ such that the first $3$ paths contain exactly 
$\lfloor\frac{k}{4}\rfloor$ real edges and the last path contains the rest. In
addition ensure that the first edge in each path is a real edge. Let the first
edge of the $4$-paths be respectively $f_0 = f'_0, f'_1, f'_2, f'_3$. We 
have the following which shows that the associated 
$4$-tuples $\left<f'_0,f'_1,f'_2,f'_3\right>$
uniquely characterise cycles in $\calC_{i+1}$.
\begin{claim}
There is at most one cycle in $\calC_{i+1}$ that has a given $4$-tuple 
$\left<f'_0,f'_1,f'_2,f'_3\right>$ associated with it.
\end{claim}
\begin{proof}
Suppose two distinct cycles $C,C' \in \calC_{i+1}$ have
a tuple $\left<f'_0,f'_1,f'_2,f'_3\right>$ 
associated with them. Then for least one $j \in \{0,1,2,3\}$
$P_j(C) \neq P_j(C')$. Then $P_j(C) \cup P_j(C')$
is a closed walk in $G_i$ containing at most 
$2\times \lceil\frac{2^{i+2}}{4}\rceil = 2^{i+1}$ many real edges,
contradicting the assumption on $G_i$.
\end{proof}

This lemma shows that there are at most $N^4$ elements in $\calC_i$.
Next consider the following lemma from \cite{FKS}:
\begin{lemma}[\cite{FKS}]
For every constant $c>0$ there is a constant $c_0>0$ such that for
every set $S$ of $m$ bit integers with $|S| \leq m^c$,
the following holds: There is a $ c_0 \log{m}$  bit prime
number $p$ such that for any $x,y \in S$ it holds that if $x \neq y$ then 
$x \not\equiv y \bmod{p}$.
\end{lemma}
We apply it to the set $c_{w_0}(\calC_i) = \{c_{w_0}(C) : C \in \calC_i\}$. 
Here, the weight
function $w_0$ assigns weights $w_0(e_j) = 2^j$ to the real edges which are
$e_1,e_2,\ldots,e_N$ in an arbitrary but fixed order.
Notice that from the above claim, the size of this set 
$|w_0(\calC_i)| \leq N^4$. % where $N$ is the number of real edges
And $w_0(e_j)$ is $j$-bits long hence $c_{w_0}(C)$ for any cycle
$C \in \calC_i$ that has less than $2^{i+2}$ real edges 
is at most $i+j+2 < 4N$-bits long.  Thus, we obtain a prime $p_{i+1}$ 
of length at most $c_0\log{4N}$ by picking $c = 4$. We define 
$w_{i+1}(e_j) = w_0(e_j) \bmod{p_{i+1}}$.

Now consider the following crucial lemma from \cite{FGT}:
\begin{lemma}[\cite{FGT}]\label{lem:crucialFGT}
Let $G = (V,E)$ be a bipartite graph with weight function $w$. 
Let $C$ be a cycle in $G$ such that $c_w(C) \neq 0$. 
Let $E_1$ be the union of all minimum weight perfect matchings in $G$.
Then the graph $G_1(V,E_1)$ does not contain the cycle $C$.
Moreover all the perfect matchings in $G_1$ have the same weight.
\end{lemma}
Let $B$ be a large enough constant (though bounded by a polynomial in $N$) 
to be specified later.
We shift the original accumulated weight function
$W_i$ and add the new weight function $w_{i+1}$ to obtain:
$W_{i+1}(e) = W_{i}(e)B + w_{i+1}(e)$. 
Apply $W_{i+1}$ on the graph $G_i$ to obtain the graph $G_{i+1}$.
 Inductively suppose we have
 the invariant~\ref{inv:analogFGT}
 that  the graph $G_i$ did not have any cycles containing at least 
$2^{i+1}$ real edges. This property is preserved when we take all the
perfect matchings in $G_i$ and apply $W_{i+1}$ yielding $G_{i+1}$. Moreover 
from Lemma~\ref{lem:crucialFGT} and the construction of $w_{i+1}$ the cycles of
$\calC_i$ disappear from $G_{i+1}$ restoring the invariant. 

Notice that it suffices to take $B$ greater than the number of real edges
times the maximum of $w_i(e)$ over $i,e$.
Showing that $G_1$ contains no cycle of length at most $4$ mimics the above
more general proof and we skip it here.
We can now complete the proof of Lemma~\ref{lem:combFGT}:
\begin{lemma*} (Lemma~\ref{lem:combFGT} restated)
Let $G$ be a bipartite graph with a non-zero circulation
$w^{old}$. Suppose $N = \log^{O(1)}{n}$ edges are inserted into $G$ to yield $G^{new}$
then we can compute polynomially many weight functions in $\FOar$ that
have $O(\log{n})$ bit weights, and at least one of them,
$w^{new}$ is isolating. Further the weights of the original edges remains
unchanged under $w^{new}$.
\end{lemma*}

\begin{proof}(of Lemma~\ref{lem:combFGT})
From the invariant above $G_\ell$ does not contain
any cycles. From the construction of $G_\ell$ if $G$ has a perfect matching then
so does $G_\ell$ and hence it is a perfect matching. Notice that $W_\ell$
is obtained from $p_1,\ldots,p_\ell$ that include $O((\log{\log{n}})^2) = o(\log{n})$ 
many bits. Thus there are (sub)polynomially many such weighting functions $W_\ell$, depending on the primes $\vec{p}$.
Let $w = B\cdot W_\ell + w^{old}$ where we recall that $W_\ell(e)$ is non-zero only
for the new (real) edges and $w^{old}$ is non-zero only for the old (fictitious)
edges. Thus, any perfect matching that consists of only old edges is lighter
than any perfect matching containing at least one new edge. Moreover if 
the real edges in two matchings differ then from the construction of 
$W_\ell$ (for some choice of $\vec{p}$) both matchings cannot be lightest 
as $W_\ell$ real isolates a matching. Thus the only remaining case is
that we have two distinct lightest perfect matchings which differ only in the
old edges. But the symmetric difference of any two such perfect matchings
is a collection of cycles consisting of old edges. But each cycle has a
non-zero circulation in the old graph and so we can obtain a matching
of even lesser weight by replacing the edges of one of the matchings in one
cycle by the edges of the other one. This contradicts that both matchings were
of least weight. This completes the proof.
\end{proof}
